# Supplementary material for: Editing Massive Concepts in Text-to-Image Diffusion Models
Source: arXiv:2403.13807 source file (2024-03-20)
Supplement: Supplementary file 1 [file supp_rectification_qualitative.tex]

\begin{figure*}[ht]
\vspace{-1em}
    \centering    
    \includegraphics[width=\linewidth]{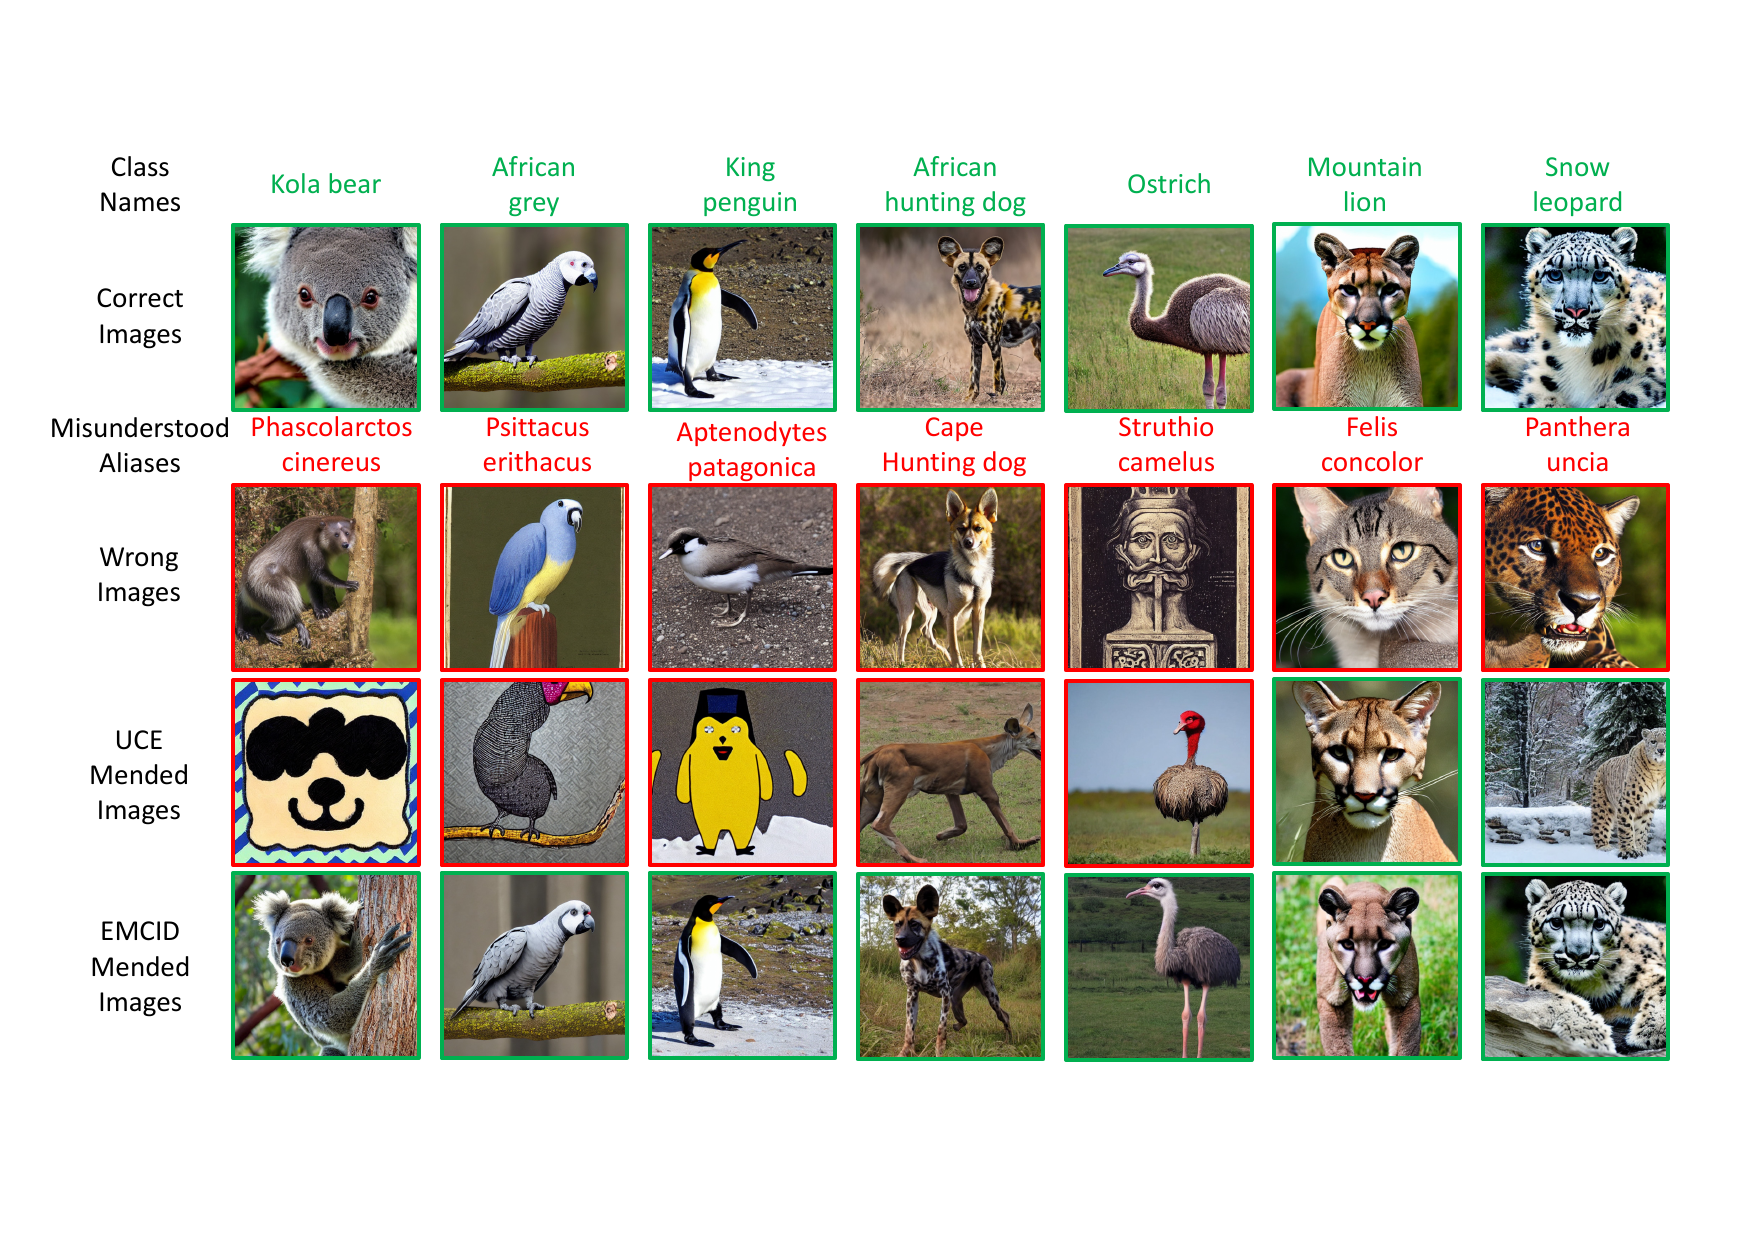}
    \vspace{-0.30in}
    \caption{
    We demonstrate more examples for the task of Concept Rectification and further compare \method{} with UCE. The 7 misunderstood aliases are rectified simultaneously with UCE and \method{} separately. Our method~(fourth row) can constantly rectify the misunderstood aliases of concepts, while UCE~(third row) often fails to succeed.
    }
    \label{fig:more rectification}
\end{figure*}
